# Supplementary material for: Towards Explainable 3D Grounded Visual Question Answering: A New Benchmark and Strong Baseline
Source: arXiv:2209.12028 source file (2022-09-24)
Supplement: Supplementary file 2 [file grounding_results.tex]

\begin{table}[t]
\caption{The grounding results of our framework on the ScanRefer~\cite{chen2020scanrefer} dataset. When joint training our FE-3DGQA dataset and the extended FE-3DGQA dataset, our method could achieve comparable results when compared with other state-of-the-art methods. We hope our work could further inspire the exploration of large-scale joint training for various 3D tasks.}
% , which further demonstrates the effectiveness of our framework
\centering
\begin{tabular}{lcccccc}
\hline
\textbf{} & \multicolumn{2}{c}{\textbf{Unique}} & \multicolumn{2}{c}{\textbf{Multiple}} & \multicolumn{2}{c}{\textbf{Overall}} \\ \hline
\multicolumn{1}{l|}{} & \multicolumn{1}{l}{Acc@0.25} & \multicolumn{1}{l}{Acc@0.5} & \multicolumn{1}{l}{Acc@0.25} & \multicolumn{1}{l}{Acc@0.5} & \multicolumn{1}{l}{Acc@0.25} & \multicolumn{1}{l}{Acc@0.5} \\ \hline
% \multicolumn{7}{c}{Validation Set (3D Only)} \\ \hline
% \multicolumn{1}{l|}{ScanRefer~\cite{chen2020scanrefer}} & 67.64 & 46.19 & 32.06 & 21.26 & 38.97 & 26.10 \\
% \multicolumn{1}{l|}{InstanceRefer~\cite{yuan2021instancerefer}} & 77.13 & \textbf{66.40} & 28.83 & 22.92 & 38.20 & 31.35 \\
% \multicolumn{1}{l|}{Non-SAT~\cite{iccv21_sat}} & 68.48 & 47.38 & 31.81 & 21.34 & 38.92 & 26.40 \\
% \multicolumn{1}{l|}{3DVG-Transformer~\cite{iccv21_3DVG-Transformer}} & 77.16 & 58.47 & 38.38 & 28.70 & 45.90 & 34.47 \\
% \multicolumn{1}{l|}{Ours} &  &  &  &  &  &  \\ \hline
% \multicolumn{7}{c}{Validation Set (2D + 3D)} \\ \hline
\multicolumn{7}{c}{Validation Set} \\ \hline
\multicolumn{1}{l|}{ScanRefer~\cite{chen2020scanrefer}} & 76.33 & 53.51 & 32.73 & 21.11 & 41.19 & 27.40 \\
\multicolumn{1}{l|}{TGNN~\cite{aaai_huang2021_TGNN}} & 68.61 & 56.80 & 29.84 & 23.18 & 37.37 & 29.70 \\
\multicolumn{1}{l|}{SAT~\cite{iccv21_sat}} & 73.21 & 50.83 & 37.64 & 25.16 & 44.54 & 30.14 \\
\multicolumn{1}{l|}{InstanceRefer~\cite{yuan2021instancerefer}} & 75.72 & \textbf{64.66} & 29.41 & 22.99 & 38.40 & 31.08 \\
\multicolumn{1}{l|}{3DVG-Transformer~\cite{iccv21_3DVG-Transformer}} & 81.93 & 60.64 & 39.30 & 28.42 & 47.57 & 34.67 \\
% \multicolumn{1}{l|}{Ours (Only ScanRefer Dataset todo)} & 81.08 & 59.02 & 36.02 & 24.61 & 44.76 & 31.29 \\ \hline
\multicolumn{1}{l|}{Ours (ScanRefer Only)} & 82.17 & 60.81 & 35.91 & 25.33 & 44.89 & 32.21 \\ \hline
% \multicolumn{1}{l|}{Ours (ScanRefer Only)} & 81.08 & 59.02 & 36.02 & 24.61 & 44.76 & 31.29 \\ \hline
% \multicolumn{1}{l|}{Ours (manual+Ext, w/o mask)} & \textbf{84.39} & \textbf{64.66} & \textbf{41.21} & 28.70 & 49.59 & 35.68 \\
\multicolumn{1}{l|}{Ours (manual+Ext.)} & \textbf{84.17} & 64.34 & \textbf{41.05} & \textbf{29.22} & \textbf{49.42} & \textbf{36.03} \\ \hline
\multicolumn{7}{c}{Online Benchmark} \\ \hline
\multicolumn{1}{l|}{ScanRefer~\cite{chen2020scanrefer}} & 68.59 & 43.53 & 34.88 & 20.97 & 42.44 & 26.03 \\
\multicolumn{1}{l|}{TGNN~\cite{aaai_huang2021_TGNN}} & 68.34 & 58.94 & 33.12 & 25.26 & 41.02 & 32.81 \\
\multicolumn{1}{l|}{InstanceRefer~\cite{yuan2021instancerefer}} & 77.82 & \textbf{66.69} & 34.57 & 26.88 & 44.27 & 35.80 \\
\multicolumn{1}{l|}{3DVG-Transformer~\cite{iccv21_3DVG-Transformer}} & 75.76 & 55.15 & 42.24 & 29.33 & 49.76 & 35.12 \\ \hline
\multicolumn{1}{l|}{Ours (manual+Ext.)} & \textbf{78.57} & 58.62 & \textbf{43.17} & \textbf{29.35} & \textbf{51.11} & \textbf{35.92} \\ \hline
\end{tabular}
\label{tab:scanrefer_result}
\end{table}

\subsection{3D Visual Grounding Datasets.}
\noindent{}For better evaluate the effectiveness of our proposed framework, we do not only evaluated the results for our methods, but report the results of single-object grounding.

% copied, should change
\noindent{}We use the ScanRefer~\cite{chen2020scanrefer} dataset to evaluate our method for the visual grounding task.
% The ScanRefer dataset built upon ScanNet dataset using $11046 $objects from $800 $scenes. There is an average of $14.14$ objects in each scene, in which each object has an average of $4.64$ descriptions, with a total of $51,583$ sentences.
The ScanRefer~\cite{chen2020scanrefer} dataset contains $51,583$ textual descriptions about $11,046$ objects from $800$ scenes. Each scene has an average of $13.81$ objects and $64.48$ descriptions.
% We follow the official ScanRefer to split this dataset as the train/val/test set, with $36,655$, $9,508$, and $5,410$ samples, respectively.
We follow the official setting to split ScanRefer~\cite{chen2020scanrefer} as the train/val/test set, with $36,655$, $9,508$, and $5,410$ samples, respectively.
% We report the overall accuracy with both``unique'' and ``multiple'' subsets for this dataset.
Following~\cite{chen2020scanrefer}, the overall accuracy and the accuracies on both``unique'' and ``multiple'' subsets are reported.
% The grounding data is labeled as ``unique'' if it only contains a single object from its class in the scene, otherwise it will be labeled as ``multiple''.
% Following~\cite{chen2020scanrefer}, 
We label each grounding data as ``unique'' if it only contains a single object from its class in the scene, otherwise it will be labeled as ``multiple''.
For this dataset, we use Acc@$0.25$IoU and Acc@$0.5$IoU as our evaluation metrics.
We also compare our method with the baseline methods on both the validation set and the online test set available at the ScanRefer's benchmark website\footnote{\url{http://kaldir.vc.in.tum.de/scanrefer\_benchmark}}.

%As a sub-dataset of ReferIt3D~\cite{eccv2020_referit3d}, Nr3D is also built based on ScanNet~\cite{dai2017scannet} with additional textual descriptions, and it contains 41,503 samples collected by ReferItGame.
%The initial task proposed for this dataset is to select which object is the preferred object, in which the object instance is given, and thus evaluated by the instance-matching accuracy.
%In this paper, we focus on the scene understanding, and use the same metric as used for performance evaluation on the ScanRefer dataset.

\subsection{3D Visual Grounding Results.}

Following ScanRefer~\cite{chen2020scanrefer}, we further report our result under the ``2D+3D'' setting (\ie, the input modality is XYZ+Multiview, corresponding to Line 3 in Table~\ref{todo}).
As shown in Tab.~\ref{tab:scanrefer_result}, our method could achieve state-of-the-art results without using various data augmentation strategies for the visual grounding task.
With more training dataset, the joint training method achieves, our method achieves more than 1.3\% and 0.7\% gains when compared with the recent SOTA method 3DVG-Transformer~\cite{iccv21_3DVG-Transformer} in terms of Acc@0.25 and Acc@0.5 metrics respectively in terms of the “overall” case on the validation set. 
%Specifically, in terms of Acc@0.25 and Acc@0.5 metrics, our method achieves around $1.9$\% and $2.6$\% improvements in the ``overall'' case when compared with 3DVG-Transformer~\cite{iccv21_3DVG-Transformer} on the validation set under the ``2D+3D'' setting.
