# Supplementary material for: Towards Explainable 3D Grounded Visual Question Answering: A New Benchmark and Strong Baseline
Source: arXiv:2209.12028 source file (2022-09-24)
Supplement: Supplementary file 3 [file different_input_type.tex]

\begin{table}[t]
\caption{Grounded question answering results when using different input modalities.}
\centering
% \caption{(a) The 3D dense captioning results on the ScanRefer Dataset}
\small
\begin{tabular}{c|ccccc|cccc}
\hline
 & \multicolumn{5}{c|}{Question Answering Results (Acc)} & \multicolumn{4}{c}{Grounding Results (AP@0.5)} \\ \cline{2-10} 
Input Modality & number & color & yes/no & other & overall & Type 1 & Type 2 & Type 3 & mean \\ \hline
xyz &  &  &  &  &  &  &  &  &  \\
xyz+rgb & 33.39 & 39.90 & 68.69 & 30.74 & 47.75 & 28.28 & 17.34 & 10.54 & 18.72 \\
xyz+multiview &  &  &  &  &  &  &  &  &  \\
xyz+rgb+multiview & 34.90 & 40.17 & 68.27 & 31.08 & 47.88 & 28.20 & 19.72 & 11.38 & 19.77 \\ \hline
\end{tabular}
\label{tab:different_training_set_result}
\end{table}

\section{The effect of different input type}

As shown in Sec.~\ref{sec:extended_gqa} our main paper, the input of our 3D vision branch is the Point Cloud $\boldsymbol{P} \in \mathbb{R}^{N\times(3+K)}$, which represents the whole scene as $N$ 3D coordinates with $K$ dimensional hidden features, which is a combination of the color, the normal vector, the height, and the 128-dimensional multi-view appearance features for each point in the 3D scene.
As shown in Table.~\ref{tab:different_training_set_result}, we further perform an ablation to evaluate the grounded visual question answering results when using different input modalities.

Tab.~\ref{tab:different_training_set_result} shows the grounded visual question answering results based on the test set of FE-3DGQA dataset when using different training datasets.
We also surprisingly found the AP result for the objects related to the answer-referred objects appeared in the question consistently improves though no extra labels for this type appear in the extended training dataset, while the grounding data improves more. We hypothesis that the referring process potentially improves the ability for the model to make a link through noun-words from the inputted language and object proposals from the scene, which benefits the QA process.
