# Supplementary material for: Towards Explainable 3D Grounded Visual Question Answering: A New Benchmark and Strong Baseline
Source: arXiv:2209.12028 source file (2022-09-24)
Supplement: Supplementary file 5 [file supplementary.tex]

% updated April 2002 by Antje Endemann
% Based on CVPR 07 and LNCS, with modifications by DAF, AZ and elle, 2008 and AA, 2010, and CC, 2011; TT, 2014; AAS, 2016; AAS, 2020; TH, 2022

\documentclass[runningheads]{llncs}
\usepackage{graphicx}
% DO NOT USE \usepackage{times}, it will be removed by typesetters
%\usepackage{times}

\usepackage{tikz}
\usepackage{comment}
\usepackage{amsmath,amssymb} % define this before the line numbering.
\usepackage{color}

\usepackage{footnote}
\makesavenoteenv{table}

% \renewcommand{\thefootnote}{${\arabic{footnote}}$}
% \newcommand\trifootnote[1]{%
% \begingroup
% \renewcommand\thefootnote{}\footnote{#1}%
% \addtocounter{footnote}{-1}%
% \endgroup
% }
% \usepackage{tikz}
% \usepackage{etoolbox}
% \newcommand*{\circled}[1]{\lower.7ex\hbox{\tikz\draw (0pt, 0pt)%
%     circle (.5em) node {\makebox[1em][c]{\small #1}};}}
% \robustify{\circled}
% \renewcommand{\thefootnote}{\circled{\value{footnote}}}

% The "axessiblity" package can be found at: https://ctan.org/pkg/axessibility?lang=en
\usepackage[accsupp]{axessibility}  % Improves PDF readability for those with disabilities.

% \def\etc{\emph{etc}.} \def\vs{\emph{vs}.}

% \newcommand{\zlc}[1]{\textcolor{black}{#1}}
% \newcommand{\zj}[1]{\textcolor{blue}{#1}}

% \newcommand{\zjn}[1]{\textcolor{blue}{#1}}

% INITIAL SUBMISSION - The following two lines are NOT commented
% CAMERA READY - Comment OUT the following two lines
\usepackage{ruler}
\usepackage[width=122mm,left=12mm,paperwidth=146mm,height=193mm,top=12mm,paperheight=217mm]{geometry}

\begin{document}
% \renewcommand\thelinenumber{\color[rgb]{0.2,0.5,0.8}\normalfont\sffamily\scriptsize\arabic{linenumber}\color[rgb]{0,0,0}}
% \renewcommand\makeLineNumber {\hss\thelinenumber\ \hspace{6mm} \rlap{\hskip\textwidth\ \hspace{6.5mm}\thelinenumber}}
% \linenumbers
\pagestyle{headings}
\mainmatter
\def\ECCVSubNumber{250}  % Insert your submission number here

% \title{3D-GQA: Free-Form Grounded Visual Question Answering On RGB-D Scans} % Replace with your title
\title{Towards Free-Form and Explainable 3D Grounded Visual Question Answering: A New Benchmark and A Strong Baseline\\\emph{Supplementary Material}} % Replace with your title
% \title{Towards Free-Form and Explainable 3D Visual Question Answering: Benchmark and Baseline} % Replace with your title

% INITIAL SUBMISSION 
%\begin{comment}
\titlerunning{ECCV-22 submission ID \ECCVSubNumber} 
\authorrunning{ECCV-22 submission ID \ECCVSubNumber} 
\author{Anonymous ECCV submission}
\institute{Paper ID \ECCVSubNumber}
%\end{comment}
%******************

% CAMERA READY SUBMISSION
\begin{comment}
\titlerunning{Abbreviated paper title}
% If the paper title is too long for the running head, you can set
% an abbreviated paper title here
%
\author{First Author\inst{1}\orcidID{0000-1111-2222-3333} \and
Second Author\inst{2,3}\orcidID{1111-2222-3333-4444} \and
Third Author\inst{3}\orcidID{2222--3333-4444-5555}}
%
\authorrunning{F. Author et al.}
% First names are abbreviated in the running head.
% If there are more than two authors, 'et al.' is used.
%
\institute{Princeton University, Princeton NJ 08544, USA \and
Springer Heidelberg, Tiergartenstr. 17, 69121 Heidelberg, Germany
\email{lncs@springer.com}\\
\url{http://www.springer.com/gp/computer-science/lncs} \and
ABC Institute, Rupert-Karls-University Heidelberg, Heidelberg, Germany\\
\email{\{abc,lncs\}@uni-heidelberg.de}}
\end{comment}
%******************
\maketitle

\renewcommand\thesection{\Alph{section}}
\setcounter{section}{0}
\setcounter{figure}{0}
\setcounter{table}{0}
\renewcommand{\thefigure}{S\arabic{figure}}
\renewcommand{\thetable}{S\arabic{table}}

\input{latex/9.supplementary/_visualizations}
\input{latex/9.supplementary/dataset_statistics}
\input{latex/9.supplementary/detailed_labeling_process}
\input{latex/9.supplementary/extended_dataset}
\input{latex/9.supplementary/extended_results}

\clearpage
% ---- Bibliography ----
%
% BibTeX users should specify bibliography style 'splncs04'.
% References will then be sorted and formatted in the correct style.
%
\bibliographystyle{splncs04}
\bibliography{egbib}
\end{document}
